# Supplementary material for: Instant Uncertainty Calibration of NeRFs Using a Meta-Calibrator
Source: arXiv:2312.02350 source file (2024-09-20)
Supplement: Supplementary file 1 [file depth-cal.tex]

\section{Depth Calibration}
\label{sec:depth}
Some NeRF models output depth estimates and corresponding uncertainties \cite{mixnerf} in addition to image predictions. However, the calibration of the derived depth confidence intervals has not been addressed. Accurate confidence intervals for depth outputs from NeRFs could enable their use as measuring tools in manufacturing and safety-critical applications where tight tolerances based on the width of confidence intervals must be met. In this section, we outline how our method could be extended to obtain calibrated confidence intervals for NeRF depth estimates. We refer the details of this framework to future work.\\

MixNeRF \cite{mixnerf} models the ray depth with a mixture of Laplacians. Therefore, in the same way that we obtained the CDF of each pixel color channel from FlipNeRF \cite{flipnerf}, we can obtain the CDF of the depth channel for each pixel from MixNeRF \cite{mixnerf} and evaluate the uncalibrated confidence levels of the ground truth depth values. Following the approach proposed in the main paper, we can construct the depth calibration curves for a set of scenes used to train the meta-calibrator. Once trained, the meta-calibrator can then be used to correct the depth confidence levels for the test scene. In this way, the framework proposed in the main paper can be extended to provide accurate confidence intervals for NeRF depth estimates.
