# Supplementary material for: Instant Uncertainty Calibration of NeRFs Using a Meta-Calibrator
Source: arXiv:2312.02350 source file (2024-09-20)
Supplement: Supplementary file 2 [file code.tex]

\section{The Code}
\label{sec:code}
We provide documented code to train the meta-calibrator to predict the PCA coefficients for the calibration curves in the file \code{train\_calibrator.py} and documented code to extract the DINOv2~\cite{oquab2023dinov2} features from the uncalibrated uncertainty maps and the inferred images in the file \code{extract\_features.py}.  We plan to release the full code for our method once the paper has been accepted.
